# Supplementary material for: Mitigating Saliency Collapse: Robust Saliency-Aware Long-Text Image-Text Alignment
Source: arXiv:2610.31005 source file (2026-10-23)
Supplement: Supplementary file 1 [file supp_differentpair.tex]

\begin{table}[htbp]
    \centering
    \caption{\textbf{Region selection experiments.} Results on INSECT and DOCCI using different local regions.}
    \label{tab:region_selection} 
    
    \resizebox{\columnwidth}{!}{
        \begin{tabular}{@{}l *{5}{c!{\color{lightlightgray}\vrule width 0.5pt}}c|*{5}{c!{\color{lightlightgray}\vrule width 0.5pt}}c @{}}
        \toprule
        \multirow{2}{*}{\shortstack[c]{\textbf{Methods}}} &
        \multicolumn{6}{c|}{\cellcolor{gray!15}\textbf{INSECT}} &
        \multicolumn{6}{c}{\cellcolor{gray!15}\textbf{DOCCI}} \\
        \cmidrule(lr){2-7}\cmidrule(lr){8-13}
        & \multicolumn{1}{c}{\cellcolor{lightpink}{R@1}} & \multicolumn{1}{c}{\cellcolor{lightpink}{R@5}} & \multicolumn{1}{c}{\cellcolor{lightpink}{R@10}}
        & \multicolumn{1}{c}{\cellcolor{lightblue}{R@1}} & \multicolumn{1}{c}{\cellcolor{lightblue}{R@5}} & \multicolumn{1}{c|}{\cellcolor{lightblue}{R@10}}
        & \multicolumn{1}{c}{\cellcolor{lightpink}{R@1}} & \multicolumn{1}{c}{\cellcolor{lightpink}{R@5}} & \multicolumn{1}{c}{\cellcolor{lightpink}{R@10}}
        & \multicolumn{1}{c}{\cellcolor{lightblue}{R@1}} & \multicolumn{1}{c}{\cellcolor{lightblue}{R@5}} & \multicolumn{1}{c}{\cellcolor{lightblue}{R@10}} \\
        \midrule
        Baseline & 8.81 
 & 24.53 & 35.41  &7.43 & 24.35 & 36.53 & 81.18  &96.67   & 98.51 & 80.00 & 96.31 &98.67 \\
        \midrule
        \rowcolor{gray!8}
        \multicolumn{13}{l}{\textit{Local Region}} \\
        Random Crop & 10.02 & 27.46 & 38.26  & 9.41 & 27.89 & 39.46 & 83.00&	97.45	&99.06	&81.98	&96.71 &	98.76 \\
        \midrule
        \rowcolor{gray!8}
        \multicolumn{13}{l}{\textit{Segmentation-based}} \\
        SAM3 & 8.98  & 26.86 & 38.34  & 8.64 & 26.25 & 37.56 & 82.86&	97.25	&99.08	&81.78&97.10	&98.67 \\
        \midrule
        \rowcolor{gray!8}
        \multicolumn{13}{l}{\textit{Saliency-based}} \\
        % ADMNet & 8.38 & 26.42 & 39.90 & 8.20 & 25.39 & 39.38 & 83.02	&97.63	&99.08	&81.33&	97.18&	98.88 \\
        FASA & \textbf{10.36}
         & \textbf{28.32} & \textbf{40.67} &\textbf{9.84} & \textbf{29.36} & \textbf{40.41} & \textbf{84.35}
         & \textbf{97.51} & \textbf{99.18} &\textbf{82.18} & \textbf{97.14} & \textbf{98.94}  \\
        \bottomrule
        \end{tabular}
    }
\end{table}
